# Supplementary material for: High-Dimensional Neural Network Potentials for Magnetic Systems Using Spin-Dependent Atom-Centered Symmetry Functions
Source: arXiv:2104.14439 source file (2021-04-29)
Supplement: Supplementary file 1 [file supplementary_information.pdf]

# Supplementary Information – High-Dimensional Neural Network Potentials for Magnetic Systems Using Spin-Dependent Atom-Centered Symmetry Functions

Marco Eckhoff[1,*] and Jörg Behler[1,2,†]

[1] *Universität Göttingen, Institut für Physikalische Chemie, Theoretische Chemie, Tammannstraße 6, 37077 Göttingen, Germany.*

[2] *Universität Göttingen, International Center for Advanced Studies of Energy Conversion (ICASEC), Tammannstraße 6, 37077 Göttingen, Germany.*

(Dated: April 29, 2021)

## I. METHODS

### A. Additional Spin-Dependent Atom-Centered Symmetry Functions

For systems in which atoms of the same element can be $M_S \neq 0$ and $M_S = 0$ the spin augmentation functions (SAF)

$$M^{0^*}(s_i, s_j) = 1 - |s_i s_j| \ , \tag{1}$$

$$M^{00^*}(s_i, s_j, s_k) = (1 - |s_i|) + |s_i| \cdot (1 - |s_j|) \cdot (1 - |s_k|) \ , \tag{2}$$

have to be used for non-magnetic interactions instead of the SAFs $M^0$ and $M^{00}$ to explicitly exclude the contributions of magnetic interactions. A radial spin-dependent atom-centered symmetry function (sACSF) containing $M^{0^*}$ includes only the **0**0, **0**+, and +0 contributions and an angular sACSF containing $M^{00^*}$ only the **0**00, **0**0+, **0**++, **0**+−, and +00 contributions shown in Figure 7 of the manuscript.

Moreover, for systems containing partly magnetically active elements, the SAFs $M^{++}$ and $M^{--}$ have to be further split to distinguish the different types of magnetic interactions,

$$M^{++2}(s_i, s_j, s_k) = \tfrac{1}{2} |s_i| \cdot (1 - |s_j s_k|) \cdot (|s_j| + |s_k|) \cdot |s_i + s_j + s_k| \ , \tag{3}$$

$$M^{++3}(s_i, s_j, s_k) = \tfrac{1}{2} |s_i s_j s_k| \cdot (|s_i + s_j + s_k| - 1) \ , \tag{4}$$

$$M^{--2}(s_i, s_j, s_k) = \tfrac{1}{2} |s_i| \cdot (1 - |s_j s_k|) \cdot (|s_j| + |s_k|) \cdot |s_i - s_j - s_k| \ , \tag{5}$$

$$M^{--3}(s_i, s_j, s_k) = \tfrac{1}{2} |s_i s_j s_k| \cdot (|s_i - s_j - s_k| - 1) \ . \tag{6}$$

The SAFs $M^{++2}$ and $M^{++3}$ separate the ++0 and +++ contributions and the SAFs $M^{--2}$ and $M^{--3}$ the +−0 and +−− contributions of the angular sACSFs shown in Figure 7 of the manuscript. For each element combination the required SAFs to include all different magnetic and non-magnetic interactions have to be employed in the construction of the magnetic high-dimensional neural network potential (mHDNNP).

The SAFs $M^{00^*}$, $M^{++2}$, $M^{--2}$, $M^{++3}$, $M^{--3}$, and $M^{+-}$ can be employed in the general case. The angular sACSFs given in Table SI yield the same description for MnO as obtained by employing the SAFs $M^{00}$, $M^{++}$, $M^{--}$, and $M^{+-}$ according to Table II of the manuscript.

TABLE SI: Alternative angular sACSFs with $\eta = 0\,a_0^{-2}$ and $R_\mathrm{c} = 10.5\,a_0$. All combinations of SAFs and symmetry function parameters are used for the given element combinations.

| ***i***-*j*-*k* | $M^{\mathrm{xx}}$ | $\lambda$ | $\zeta$ |
|---|---|---|---|
| **O**-O-O | $M^{00^*}$ | −1, 1 | 1, 2, 4, 16 |
| **O**-O-Mn | $M^{00^*}$ | −1, 1 | 1, 2, 4, 16 |
| **O**-Mn-Mn | $M^{00^*}$ | −1, 1 | 1, 2, 4, 16 |
| **Mn**-O-O | $M^{00^*}$ | −1, 1 | 1, 2, 4, 16 |
| **Mn**-O-Mn | $M^{++2}$, $M^{--2}$ | −1, 1 | 1, 2, 4, 16 |
| **Mn**-Mn-Mn | $M^{++3}$, $M^{--3}$, $M^{+-}$ | −1, 1 | 1, 2, 4, 16 |

## II. COMPUTATIONAL DETAILS

### A. Construction of the Reference Data Set

The initial reference data set was based on the experimentally determined MnO crystal structure. For $Mn_{0.969}O$ structures one Mn atom was removed from the $2 \times 2 \times 2$ MnO supercell and a density functional theory (DFT) geometry optimization was performed. Random displacements of the atomic positions inside spheres with radii of up to 0.2 Å and scaling of the lattice constants by up to ±3% were applied to mimic thermal distortions and to obtain a set of configurations. Configurations with O-O distances smaller than 2.4 Å, O-Mn distances smaller than 1.6 Å, and Mn-Mn distances smaller than 2.45 Å were discarded. The magnetic orders were derived from the AFM-II and FM orders in which the spins were flipped with a probability of 0, 12.5, 25, 37.5, or 50%. The energy and forces were calculated for each configuration employing DFT. Configurations with a cohesive energy (energy of the system minus the sum of the atomic energies of O in the $^3P_2$ state and Mn in the $^6S_{5/2}$ state) larger than $-5.0\,\mathrm{eV\,atom^{-1}}$ and atomic forces larger than $2.5\,\mathrm{eV}\,a_0^{-1}$ for O and $3.0\,\mathrm{eV}\,a_0^{-1}$ for Mn were not included in the reference data set as well

* marco.eckhoff@chemie.uni-goettingen.de
† joerg.behler@uni-goettingen.de

as configurations including Hirshfeld spin moments of O outside the interval $[0.0, 0.225]$ and Mn outside the interval $[1.7, 2.45]$.

A preliminary mHDNNP can be trained on this initial reference data set. mHDNNP-driven $NpT$ molecular dynamics (MD) simulations enable to sample the geometric configuration space accessible at a given temperature. The magnetic configurations can be explored by including a spin-flip of a randomly chosen Mn atom after every 10 MD steps. Employing these simulations missing configurations in the reference data set can be obtained in two ways:

If the values of the sACSFs exceed the trained configuration space, the corresponding configuration is not included. If the sum of the normalized sACSF extrapolations,

$$\Delta G = \sum_{\substack{G_i < G_i^{\min} \\ \vee G_i > G_i^{\max}}} \left| \frac{G_i - G_i^{\min}}{G_i^{\max} - G_i^{\min}} - \frac{1}{2} \right| - \frac{1}{2} \ , \qquad (7)$$

with the sACSFs values $G_i$ and the corresponding minimum and maximum sACSFs values in the training set $G_i^{\min}$ and $G_i^{\max}$, is above a threshold, the configuration is recalculated using DFT and added to the reference data set. A second higher threshold supports a faster expansion of the reference data set. Adjusting these thresholds depending on the fraction of simulations showing extrapolations and on the time step separation between the additional reference structures as well as their structural deformation is essential for an efficient training.

Configurations inside the trained sACSF space but too distant from training data have to be added to the reference data set as well. These configurations lead to deviations in energy and forces predictions between different mHDNNPs trained to the same reference data set but using, for example, different neural network architectures and initial weights. However, these deviations can be employed to identify the missing configurations in the reference data set [1]. Uncorrelated configurations from the MD simulations with deviations above a predefined threshold, i.e., with large interpolation errors, can be recalculated using DFT and added to the reference data set. Subsequently, the extended reference data set can be used to train an improved mHDNNP. By repeating this self-learning process several times the sampling of the accessible configuration space can be completed to obtain a reliable mHDNNP. For an efficient training different structures of the reference data set should be used as initial structures in the MD simulations with different initial velocity distributions. Employing also temperatures in the MD simulations which are higher than the temperature range of the intended production simulations can speed-up the training process.

The RuNNerActiveLearn program package automatizes the process of finding missing structures. It is now freely available under the GPL3 license in the RuNNer repository at gitlab [2, 3]. RuNNerActiveLearn has been applied in the generation of the reference data set of this work and its previous versions were also successfully applied in References [4] and [5].

The numerical consistency of the reference data set has been monitored by analyzing the correlation between the errors of all data points obtained in different mHDNNPs [5].

### B. FHI-aims Settings

The general settings of the FHI-aims DFT calculations are given in Table SII. The basis set specification for O and Mn atoms is summarized in Table SIII. Geometry optimizations were performed with the additional settings "relax_geometry bfgs 1.0E−3", "relax_unit_cell full", and "max_relaxation_steps 25". In case of the restricted optimizations to obtain the optimized cubic AFM-II configuration "relax_unit_cell fixed_angles" was applied.

TABLE SII: Settings of the FHI-aims DFT calculations.

| Keyword | Setting |
|---|---|
| charge | 0.0 |
| spin | collinear |
| relativistic | atomic_zora scalar |
| xc | hse06 0.11 |
| hse_unit | b |
| sc_accuracy_rho | 1.0E−5 |
| sc_accuracy_eev | 1.0E−3 |
| sc_accuracy_etot | 1.0E−6 |
| sc_accuracy_forces | 1.0E−4 |
| sc_iter_limit | 250 |
| k_grid | 2 2 2 |
| KS_method | parallel |
| RI_method | LVL_fast |
| density_update_method | density_matrix |
| packed_matrix_format | index |
| collect_eigenvectors | .false. |
| distributed_spline_storage | .true. |
| use_local_index | .true. |
| load_balancing | .true. |
| use_ovlp_swap | |
| use_2d_corr | .false. |
| output k_eigenvalue | 1 |
| output | hirshfeld |

### C. RuNNer Settings

The settings of the RuNNer mHDNNP fits are given in Table SIV. The settings of the employed symmetry functions are provided in Tables I and II of the manuscript. The initial weights were obtained using the modified Xavier initialization described in our previous work [5].

TABLE SIII: Basis set specification for O and Mn atoms.

| Keyword | O | Mn |
|---|---|---|
| species | O | Mn |
| nucleus | 8 | 25 |
| mass | 15.9994 | 54.938045 |
| l_hartree | 6 | 6 |
| cut_pot | 4.0 2.0 1.0 | 4.0 2.0 1.0 |
| basis_dep_cutoff | 1E−4 | 1E−4 |
| radial_base | 36 7.0 | 50 7.0 |
| radial_multiplier | 2 | 2 |
| angular_grids | specified | specified |
| division | 0.1817 50 | 0.2623 50 |
| division | 0.3417 110 | 0.5927 110 |
| division | 0.4949 194 | 0.9156 194 |
| division | 0.6251 302 | 1.1008 302 |
| division | 0.8014 434 | 1.2671 434 |
| outer_grid | 434 | 434 |
| valence | 2 s 2. | 4 s 2. |
| valence | 2 p 4. | 3 p 6. |
| valence | | 3 d 5. |
| ion_occ | 2 s 1. | 4 s 1. |
| ion_occ | 2 p 3. | 3 p 6. |
| ion_occ | | 3 d 4. |
| hydro | 2 p 1.8 | 4 f 9.6 |
| hydro | 3 d 7.6 | 3 d 3.2 |
| hydro | 3 s 6.4 | 2 p 2 |
| hydro | 4 f 11.6 | 3 s 3.3 |

TABLE SIV: Settings of the RuNNer mHDNNP fits excluding the symfunction_short settings. A modified version of RuNNer version 1.0 has been used including the implementation of sACSFs.

| Keyword | Setting |
|---|---|
| runner_mode | 1/2 |
| nn_type_short | 1 |
| parallel_mode | 1 |
| random_number_type | 6 |
| random_seed | 227 |
| number_of_elements | 2 |
| elements | O Mn |
| remove_atom_energies | |
| atom_energy | O −75.0622724 |
| atom_energy | Mn −1162.6706313 |
| use_short_nn | |
| global_hidden_layers_short | 3 |
| global_nodes_short | 20 15 10 |
| global_activation_short | t t t l |
| test_fraction | 0.1 |
| cutoff_type | 1 |
| epochs | 30 |
| points_in_memory | 3500 |
| mix_all_points | |
| scale_symmetry_functions | |
| center_symmetry_functions | |
| fitting_unit | eV |
| use_old_weights_short | |
| use_short_forces | |
| optmode_short_energy | 1 |
| optmode_short_force | 1 |
| kalman_lambda_short | 0.98 |
| kalman_nue_short | 0.9987 |
| short_energy_fraction | 1.0 |
| short_force_fraction | 0.15 |
| short_energy_error_threshold | 0.0 |
| short_force_error_threshold | 0.5 |
| repeated_energy_update | |
| force_update_scaling | 1.5 |
| write_weights_epoch | 1 |
| write_trainpoints | |
| write_trainforces | |

## III. RESULTS

### A. Radial Distribution Functions

Two equally stable structures exist for the cubic MnO lattice: The AFM-II configuration and a second antiferromagnetic configuration shown in Figure 2 (a) and (b) in the manuscript. The radial distribution functions $g(r)$ between ferro- and antiferromagnetically interacting Mn ions in Figure S1 (a) and (b) show that the same ferro- and antiferromagnetic interactions are present in both configurations explaining their degeneracy.

### B. Pressure Dependent Structural Changes

Restriction-free optimizations at pressures from $-7$ to 7 GPa in steps of 1 GPa of the AFM-II and 1000 different PM configurations, which were obtained during the 10 ns $NpT$ MD simulation including Monte Carlo spin-flips (MDMC) of a $6\times6\times6$ MnO supercell at 400 K, were performed. The energy-volume relation can be described by the Birch-Murnaghan equation of state [6, 7],

$$E = E_0 + \frac{9B_0V_0}{16N_{\mathrm{cell}}}\left[\left(\frac{V_0}{V}\right)^{\frac{2}{3}}-1\right]^2\left\{B_0'\left[\left(\frac{V_0}{V}\right)^{\frac{2}{3}}-1\right]-4\left(\frac{V_0}{V}\right)^{\frac{2}{3}}+6\right\}, \tag{8}$$

with the energy per atom $E$, the lattice volume per unit cell $V$, the number of atoms per unit cell $N_{\mathrm{cell}}$, and the zero pressure quantities of the energy $E_0$, volume $V_0$, bulk modulus $B_0$, and pressure derivative of the bulk modulus $B_0'$.

The bulk modulus of the AFM-II configuration $B_0^{\text{AFM-II}} = 164\,\text{GPa}$ and the PM configuration $B_0^{\text{PM}} = 163\,\text{GPa}$ are similar. Since the volume at zero pressure

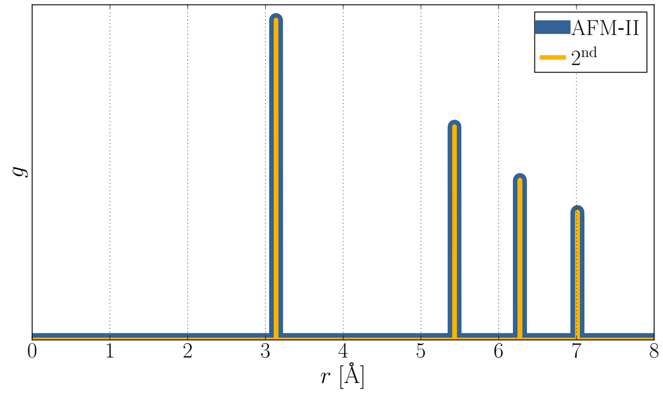


(a)

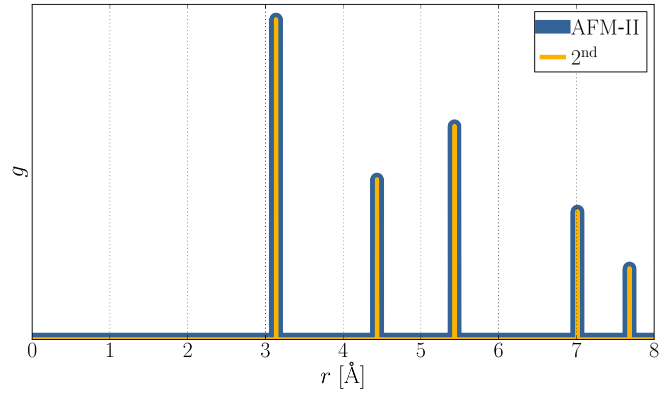


(b)

FIG. S1: Radial distribution function $g(r)$ between (a) ferromagnetically and (b) antiferromagnetically interacting Mn ions in both stable cubic configurations.

$V_0$ is smaller for AFM-II than PM, the energy difference between AFM-II and PM decreases for $\sqrt[3]{V} > 4.435$ Å as shown in the energy-volume relation in Figure S2.

### C. Temperature Dependent Structural Changes

The mHDNNP-optimized AFM-II configuration shows a rhombohedral distortion of 0.77 °. From the MDMC simulations we obtain that the distortion increases very slightly with increasing temperature up to about the half Néel temperature where it starts to decrease again (Figure S3). At the Néel temperature it drops to 0 °, since the optimized PM configurations are on average cubic.

The volumetric thermal expansion coefficient,

$$\alpha_V(T) = \frac{1}{V(T)} \left( \frac{\mathrm{d}V(T)}{\mathrm{d}T} \right)_p , \tag{9}$$

of the PM configuration calculated by the mHDNNP is $\alpha_\mathrm{V}^\mathrm{mHDNNP} = 43 \cdot 10^{-6}\,\mathrm{K}^{-1}$ at 400 K. In experiment it is determined to be $\alpha_\mathrm{V}^\mathrm{exp} = 37 \cdot 10^{-6}\,\mathrm{K}^{-1}$ at 400 K [8].

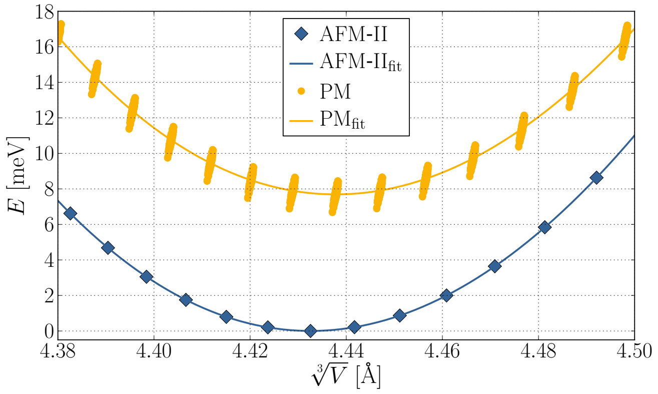


FIG. S2: Energy per atom $E$ as a function of the cube root of the lattice volume per unit cell $\sqrt[3]{V}$ obtained in optimizations at various pressures of the MnO AFM-II configuration and 1000 PM configurations, which were initialized from configurations of the MDMC simulation at 400 K. The data points are fitted using the Birch-Murnaghan equation of state [6, 7].

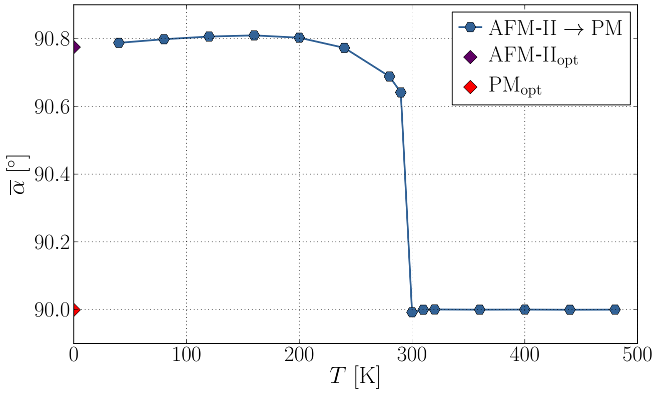


FIG. S3: Mean lattice angle $\overline{\alpha}$ as a function of the temperature $T$ obtained in MDMC simulations as well as the optimized lattice angles of the AFM-II and PM configuration.

### D. Heat Capacity of Defect Structures

The transition temperature as a function of the Mn vacancy concentration in $Mn_xO$ can be obtained from peaks in the heat capacity at constant pressure $C_p$. In Figure S4 peaks at $(298 \pm 1)$ K for $x = 1$, $(296 \pm 1)$ K for $x = 0.999$, $(274 \pm 1)$ K for $x = 0.991$, and $(234 \pm 1)$ K for $x = 0.969$ can be obtained. According to Figure 6 in the manuscript all peaks can be assigned to the AFM-II to PM transition with the Néel temperatures $(298 \pm 1)$ K for $x = 1$, $(296 \pm 1)$ K for $x = 0.999$, $(275 \pm 1)$ K for $x = 0.991$, and $(235 \pm 1)$ K for $x = 0.969$.

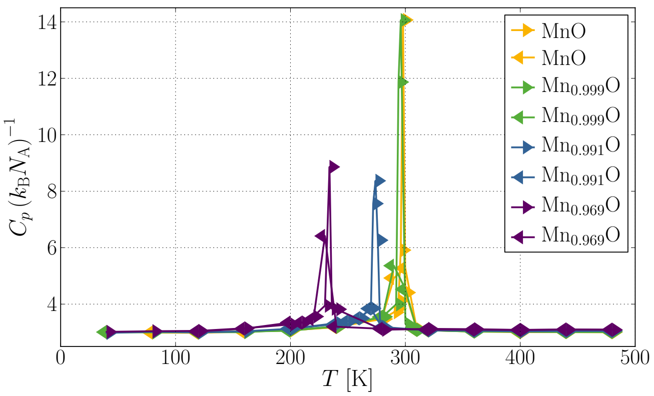


FIG. S4: Heat capacity at constant pressure $C_p$ as a function of the temperature $T$ obtained in MDMC simulations for $6 \times 6 \times 6$ supercells of MnO, $Mn_{0.999}O$, $Mn_{0.991}O$, and $Mn_{0.969}O$.

### E. Optimized Structures

The mHDNNP-optimized MnO structures of the rhombohedral global minimum AFM-II configuration and the second cubic global minimum configuration are given in Tables SV and SVI. The geometric structure of the cubic global minimum AFM-II configuration is identical to the geometric structure of the second cubic global minimum configuration.


[1] Artrith, N. & Behler, J. High-dimensional neural network potentials for metal surfaces: A prototype study for copper. *Phys. Rev. B* **85**, 045439 (2012).

[2] Behler, J. The RuNNer code. *https://www.uni-goettingen.de/en/560580.html* (April 28, 2021).

[3] Behler, J. RuNNer. *http://gitlab.com/TheochemGoettingen/RuNNer* (July 10, 2019).

[4] Eckhoff, M. & Behler, J. From molecular fragments to the bulk: Development of a neural network potential for MOF-5. *J. Chem. Theory Comput.* **15**, 3793–3809 (2019).

[5] Eckhoff, M. *et al.* Closing the gap between theory and experiment for lithium manganese oxide spinels using a high-dimensional neural network potential. *Phys. Rev. B* **102**, 174102 (2020).

[6] Murnaghan, F. D. Finite deformations of an elastic solid. *Am. J. Math.* **59**, 235–260 (1937).

[7] Birch, F. Finite elastic strain of cubic crystals. *Phys. Rev.* **71**, 809–824 (1947).

[8] Suzuki, I., Okajima, S.-I. & Seya, K. Thermal expansion of single-crystal manganosite. *J. Phys. Earth* **27**, 63–69 (1979).

TABLE SV: Rhombohedral global minimum AFM-II configuration of MnO with lattice parameters $a = 8.86595\,\text{Å}$ and $\alpha = 90.77495\,^{\circ}$.

| Element | $x$ / Å | $y$ / Å | $z$ / Å | $s$ |
|---|---|---|---|---|
| O | −0.02998 | −0.03039 | 2.21608 | 0 |
| O | −0.08993 | −0.09116 | 6.64823 | 0 |
| O | −0.02998 | 2.21629 | 0.00000 | 0 |
| O | −0.08993 | 2.15551 | 4.43215 | 0 |
| O | −0.08993 | 4.40218 | 2.21608 | 0 |
| O | −0.14989 | 4.34141 | 6.64823 | 0 |
| O | −0.08993 | 6.64886 | 0.00000 | 0 |
| O | −0.14989 | 6.58808 | 4.43215 | 0 |
| O | 2.21649 | 0.00000 | 0.00000 | 0 |
| O | 2.15653 | −0.06077 | 4.43215 | 0 |
| O | 2.15653 | 2.18590 | 2.21608 | 0 |
| O | 2.09658 | 2.12513 | 6.64823 | 0 |
| O | 2.15653 | 4.43257 | 0.00000 | 0 |
| O | 2.09658 | 4.37180 | 4.43215 | 0 |
| O | 2.09658 | 6.61847 | 2.21608 | 0 |
| O | 2.03662 | 6.55770 | 6.64823 | 0 |
| O | 4.40300 | −0.03039 | 2.21608 | 0 |
| O | 4.34304 | −0.09116 | 6.64823 | 0 |
| O | 4.40300 | 2.21629 | 0.00000 | 0 |
| O | 4.34304 | 2.15551 | 4.43215 | 0 |
| O | 4.34304 | 4.40218 | 2.21608 | 0 |
| O | 4.28309 | 4.34141 | 6.64823 | 0 |
| O | 4.34304 | 6.64886 | 0.00000 | 0 |
| O | 4.28309 | 6.58808 | 4.43215 | 0 |
| O | 6.64946 | 0.00000 | 0.00000 | 0 |
| O | 6.58951 | −0.06077 | 4.43215 | 0 |
| O | 6.58951 | 2.18590 | 2.21608 | 0 |
| O | 6.52955 | 2.12513 | 6.64823 | 0 |
| O | 6.58951 | 4.43257 | 0.00000 | 0 |
| O | 6.52955 | 4.37180 | 4.43215 | 0 |
| O | 6.52955 | 6.61847 | 2.21608 | 0 |
| O | 6.46960 | 6.55770 | 6.64823 | 0 |
| Mn | 0.00000 | 0.00000 | 0.00000 | 1 |
| Mn | −0.11991 | 2.12513 | 6.64823 | 1 |
| Mn | −0.11991 | 4.37180 | 4.43215 | 1 |
| Mn | −0.11991 | 6.61847 | 2.21608 | 1 |
| Mn | 2.12655 | −0.09116 | 6.64823 | 1 |
| Mn | 2.12655 | 2.15551 | 4.43215 | 1 |
| Mn | 2.12655 | 4.40218 | 2.21608 | 1 |
| Mn | 2.12655 | 6.64886 | 0.00000 | 1 |
| Mn | 4.37302 | −0.06077 | 4.43215 | 1 |
| Mn | 4.37302 | 2.18590 | 2.21608 | 1 |
| Mn | 4.37302 | 4.43257 | 0.00000 | 1 |
| Mn | 4.25311 | 6.55770 | 6.64823 | 1 |
| Mn | 6.61949 | −0.03039 | 2.21608 | 1 |
| Mn | 6.61949 | 2.21629 | 0.00000 | 1 |
| Mn | 6.49957 | 4.34141 | 6.64823 | 1 |
| Mn | 6.49957 | 6.58808 | 4.43215 | 1 |
| Mn | −0.05996 | −0.06077 | 4.43215 | −1 |
| Mn | −0.05996 | 2.18590 | 2.21608 | −1 |
| Mn | −0.05996 | 4.43257 | 0.00000 | −1 |
| Mn | −0.17987 | 6.55770 | 6.64823 | −1 |
| Mn | 2.18651 | −0.03039 | 2.21608 | −1 |
| Mn | 2.18651 | 2.21629 | 0.00000 | −1 |
| Mn | 2.06660 | 4.34141 | 6.64823 | −1 |
| Mn | 2.06660 | 6.58808 | 4.43215 | −1 |
| Mn | 4.43298 | 0.00000 | 0.00000 | −1 |
| Mn | 4.31306 | 2.12513 | 6.64823 | −1 |
| Mn | 4.31306 | 4.37180 | 4.43215 | −1 |
| Mn | 4.31306 | 6.61847 | 2.21608 | −1 |
| Mn | 6.55953 | −0.09116 | 6.64823 | −1 |
| Mn | 6.55953 | 2.15551 | 4.43215 | −1 |
| Mn | 6.55953 | 4.40218 | 2.21608 | −1 |
| Mn | 6.55953 | 6.64886 | 0.00000 | −1 |

TABLE SVI: Second cubic global minimum configuration of MnO with lattice parameter $a = 8.86872\,\text{Å}$.

| Element | $x$ / Å | $y$ / Å | $z$ / Å | $s$ |
|---|---|---|---|---|
| O | 0.00000 | 0.00000 | 2.21718 | 0 |
| O | 0.00000 | 0.00000 | 6.65154 | 0 |
| O | 0.00000 | 2.21718 | 0.00000 | 0 |
| O | 0.00000 | 2.21718 | 4.43436 | 0 |
| O | 0.00000 | 4.43436 | 2.21718 | 0 |
| O | 0.00000 | 4.43436 | 6.65154 | 0 |
| O | 0.00000 | 6.65154 | 0.00000 | 0 |
| O | 0.00000 | 6.65154 | 4.43436 | 0 |
| O | 2.21718 | 0.00000 | 0.00000 | 0 |
| O | 2.21718 | 0.00000 | 4.43436 | 0 |
| O | 2.21718 | 2.21718 | 2.21718 | 0 |
| O | 2.21718 | 2.21718 | 6.65154 | 0 |
| O | 2.21718 | 4.43436 | 0.00000 | 0 |
| O | 2.21718 | 4.43436 | 4.43436 | 0 |
| O | 2.21718 | 6.65154 | 2.21718 | 0 |
| O | 2.21718 | 6.65154 | 6.65154 | 0 |
| O | 4.43436 | 0.00000 | 2.21718 | 0 |
| O | 4.43436 | 0.00000 | 6.65154 | 0 |
| O | 4.43436 | 2.21718 | 0.00000 | 0 |
| O | 4.43436 | 2.21718 | 4.43436 | 0 |
| O | 4.43436 | 4.43436 | 2.21718 | 0 |
| O | 4.43436 | 4.43436 | 6.65154 | 0 |
| O | 4.43436 | 6.65154 | 0.00000 | 0 |
| O | 4.43436 | 6.65154 | 4.43436 | 0 |
| O | 6.65154 | 0.00000 | 0.00000 | 0 |
| O | 6.65154 | 0.00000 | 4.43436 | 0 |
| O | 6.65154 | 2.21718 | 2.21718 | 0 |
| O | 6.65154 | 2.21718 | 6.65154 | 0 |
| O | 6.65154 | 4.43436 | 0.00000 | 0 |
| O | 6.65154 | 4.43436 | 4.43436 | 0 |
| O | 6.65154 | 6.65154 | 2.21718 | 0 |
| O | 6.65154 | 6.65154 | 6.65154 | 0 |
| Mn | 0.00000 | 0.00000 | 0.00000 | −1 |
| Mn | 0.00000 | 2.21718 | 6.65154 | 1 |
| Mn | 0.00000 | 4.43436 | 4.43436 | −1 |
| Mn | 0.00000 | 6.65154 | 2.21718 | 1 |
| Mn | 2.21718 | 0.00000 | 6.65154 | 1 |
| Mn | 2.21718 | 2.21718 | 4.43436 | 1 |
| Mn | 2.21718 | 4.43436 | 2.21718 | 1 |
| Mn | 2.21718 | 6.65154 | 0.00000 | 1 |
| Mn | 4.43436 | 0.00000 | 4.43436 | −1 |
| Mn | 4.43436 | 2.21718 | 2.21718 | 1 |
| Mn | 4.43436 | 4.43436 | 0.00000 | −1 |
| Mn | 4.43436 | 6.65154 | 6.65154 | 1 |
| Mn | 6.65154 | 0.00000 | 2.21718 | 1 |
| Mn | 6.65154 | 2.21718 | 0.00000 | 1 |
| Mn | 6.65154 | 4.43436 | 6.65154 | 1 |
| Mn | 6.65154 | 6.65154 | 4.43436 | 1 |
| Mn | 0.00000 | 0.00000 | 4.43436 | 1 |
| Mn | 0.00000 | 2.21718 | 2.21718 | −1 |
| Mn | 0.00000 | 4.43436 | 0.00000 | 1 |
| Mn | 0.00000 | 6.65154 | 6.65154 | −1 |
| Mn | 2.21718 | 0.00000 | 2.21718 | −1 |
| Mn | 2.21718 | 2.21718 | 0.00000 | −1 |
| Mn | 2.21718 | 4.43436 | 6.65154 | −1 |
| Mn | 2.21718 | 6.65154 | 4.43436 | −1 |
| Mn | 4.43436 | 0.00000 | 0.00000 | 1 |
| Mn | 4.43436 | 2.21718 | 6.65154 | −1 |
| Mn | 4.43436 | 4.43436 | 4.43436 | 1 |
| Mn | 4.43436 | 6.65154 | 2.21718 | −1 |
| Mn | 6.65154 | 0.00000 | 6.65154 | −1 |
| Mn | 6.65154 | 2.21718 | 4.43436 | −1 |
| Mn | 6.65154 | 4.43436 | 2.21718 | −1 |
| Mn | 6.65154 | 6.65154 | 0.00000 | −1 |
